# Supplementary material for: Evolutionary Planning in Latent Space
Source: arXiv:2011.11293 source file (2020-11-23)
Supplement: Supplementary file 1 [file 8_appendix.tex]

\section{Appendix}
\subsubsection{Experiment results}
%\begin{table}[ht]
%    \centering
%    \begin{tabular}{l|r}
%        Model & Mean reward \\\hline
 %       Expert & $765.17 \pm 102.18$ \\
  %      Random & $356.20 \pm 176.6$  
  %  \end{tabular}
  %  \caption{\label{tab:havsrandom}CarRacing-v0 mean reward over 100 trials achieved using MDN-RNN trained on random rollouts and a mixture of expert and random rollouts.}
%\end{table}
\begin{table}[ht]
    \centering
    \begin{tabular}{l|r}
        Iteration & Mean reward \\\hline
        0  & $383.75 \pm 183.68$ \\
        1  & $557.87 \pm 244.97$ \\
        2  & $623.05 \pm 242.27$ \\
        3  & $618.05 \pm 231.37$ \\
        4  & $655.07 \pm 228.27$ \\
        5  & $656.83 \pm 226.67$
        % 6  & $641.43 \pm 234.07$ \\
        % 7  & $677.65 \pm 200.68$ \\
        % 8  & $664.95 \pm 235.92$ \\
        % 9  & $665.58 \pm 228.25$ \\
        % 10 & $678.55 \pm 210.09$
    \end{tabular}
    \caption{\label{tab:exp_a}CarRacing-v0 mean reward over 100 trials for iterative experiment}
\end{table}
% \begin{table}[ht]
%     \centering
%     \begin{tabular}{l|r}
%         Iteration & Mean reward \\\hline
%         0 & $339.14 \pm 159.03$ \\
%         1 & $483.57 \pm 233.65$ \\
%         \textbf{2} & $\textbf{626.20} \pm \textbf{218.36}$ \\
%         3 & $501.17 \pm 241.48$
%     \end{tabular}
%     \caption{\label{tab:exp_b}CarRacing-v0 mean iteration reward over 100 trials for experiment B}
% \end{table}
\begin{table}[ht]
    \centering
    \begin{tabular}{l|r}
        Generations & Mean reward \\\hline
        5&$473.53 \pm 280.18$\\
        10&$656.83 \pm 226.67$\\
        15&$707.79 \pm 195.44$\\
        20&$690.51 \pm 230.34$\\
        25&$669.24 \pm 208.48$\\
        30&$676.07 \pm 215.89$
    \end{tabular}
    \caption{\label{tab:exp_gen}CarRacing-v0 mean iteration reward over 100 trials with different max generation values}
\end{table}
\begin{table}[ht]
    \centering
    \begin{tabular}{l|r}
        Horizon & Mean reward \\\hline
            5  & $31.91\pm 40.54$ \\
            10 & $431.06\pm 298.79$ \\
            15 & $645.53\pm 223.84$ \\
            20 & $656.83\pm226.67$ \\
            25 & $660.48\pm 227.63 $ \\
            30 & $625.33\pm177.79$
    \end{tabular}
    \caption{\label{tab:exp_hor}CarRacing-v0 mean iteration reward over 100 trials with different horizon lengths}
\end{table}
